# Supplementary material for: Interactively shaping robot behaviour with unlabeled human instructions
Source: arXiv:1902.01670 ancillary file (2020-11-24)
Supplement: Supplementary file 1 [file Supplementary_material.pdf]

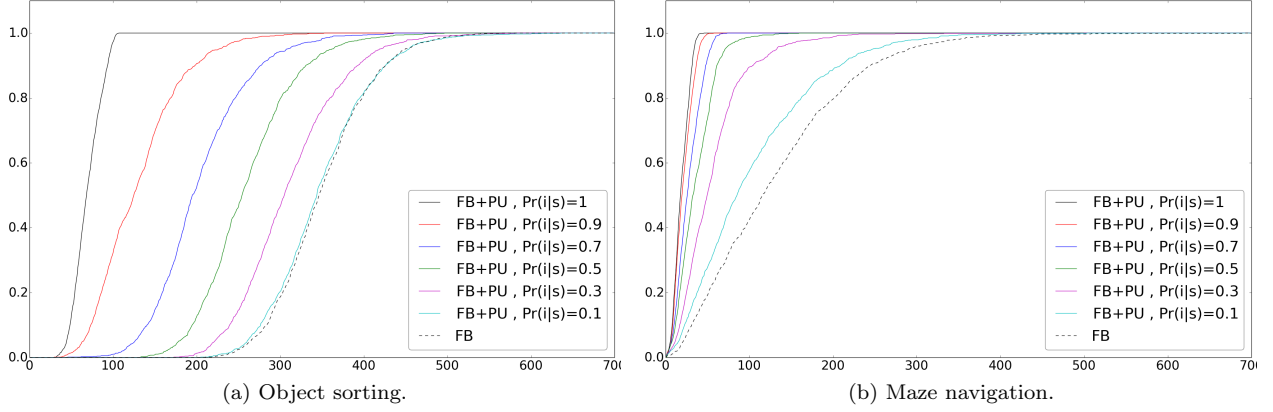

Figure 1: Learning from evaluative feedback, sparse instructions. Probability to converge before  $n$  steps. Lines from black to cyan: probability of instructions from 1 to 0.1. Dashed line: baseline model.

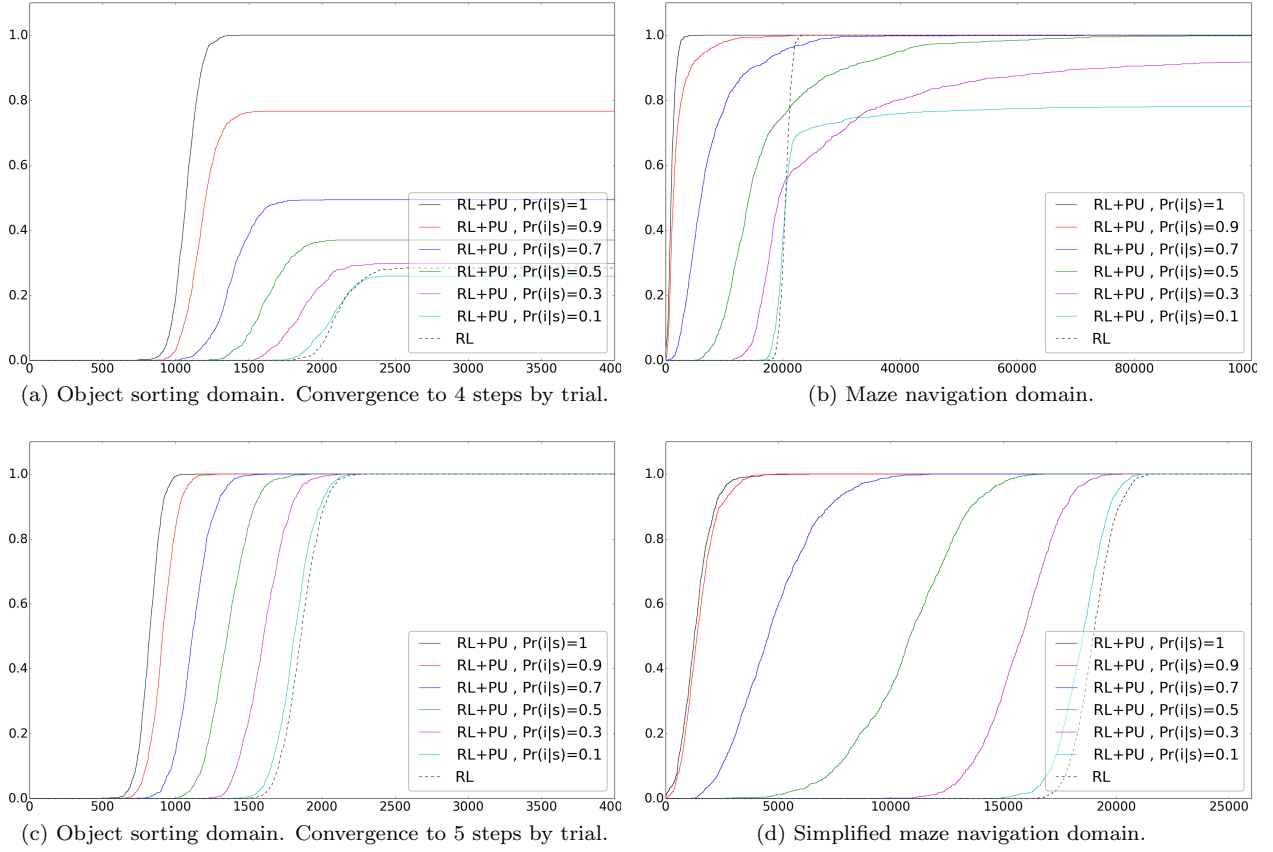

Figure 2: Learning from a predefined reward function, sparse instructions. Probability to converge before  $n$  steps. Lines from black to cyan: probability of instructions from 1 to 0.1. Dashed line: baseline model.

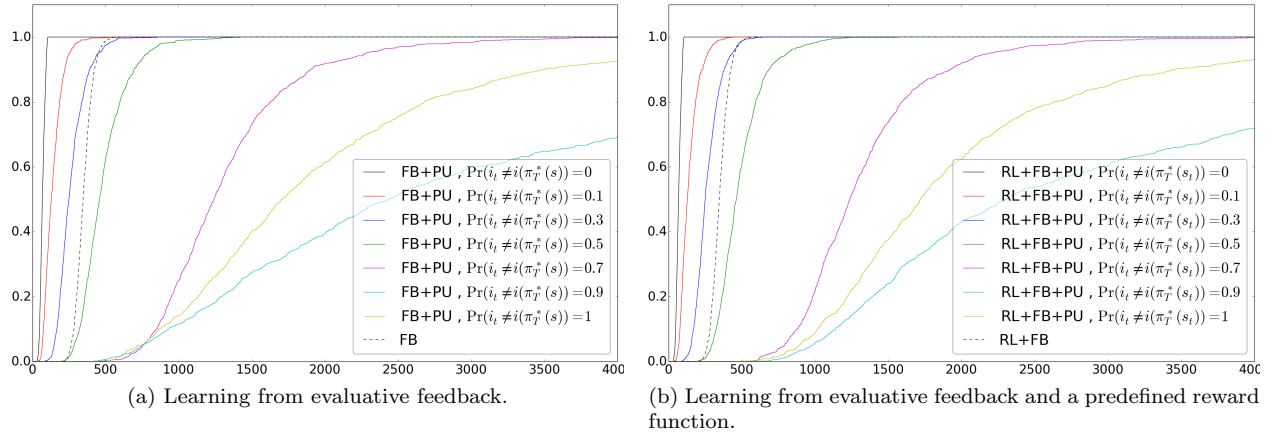

Figure 3: Shaping with erroneous instructions. Object sorting domain. Probability to converge before  $n$  steps. Lines from black to yellow: probability of erroneous instructions from 0 to 1. Dashed black: baseline model.
